# Supplementary material for: Modeling solvation effects in real-space and real-time within Density Functional Approaches
Source: arXiv:1507.05471 source file (2015-07-20)
Supplement: Supplementary file 1 [file figs_supplemental_material.pdf]

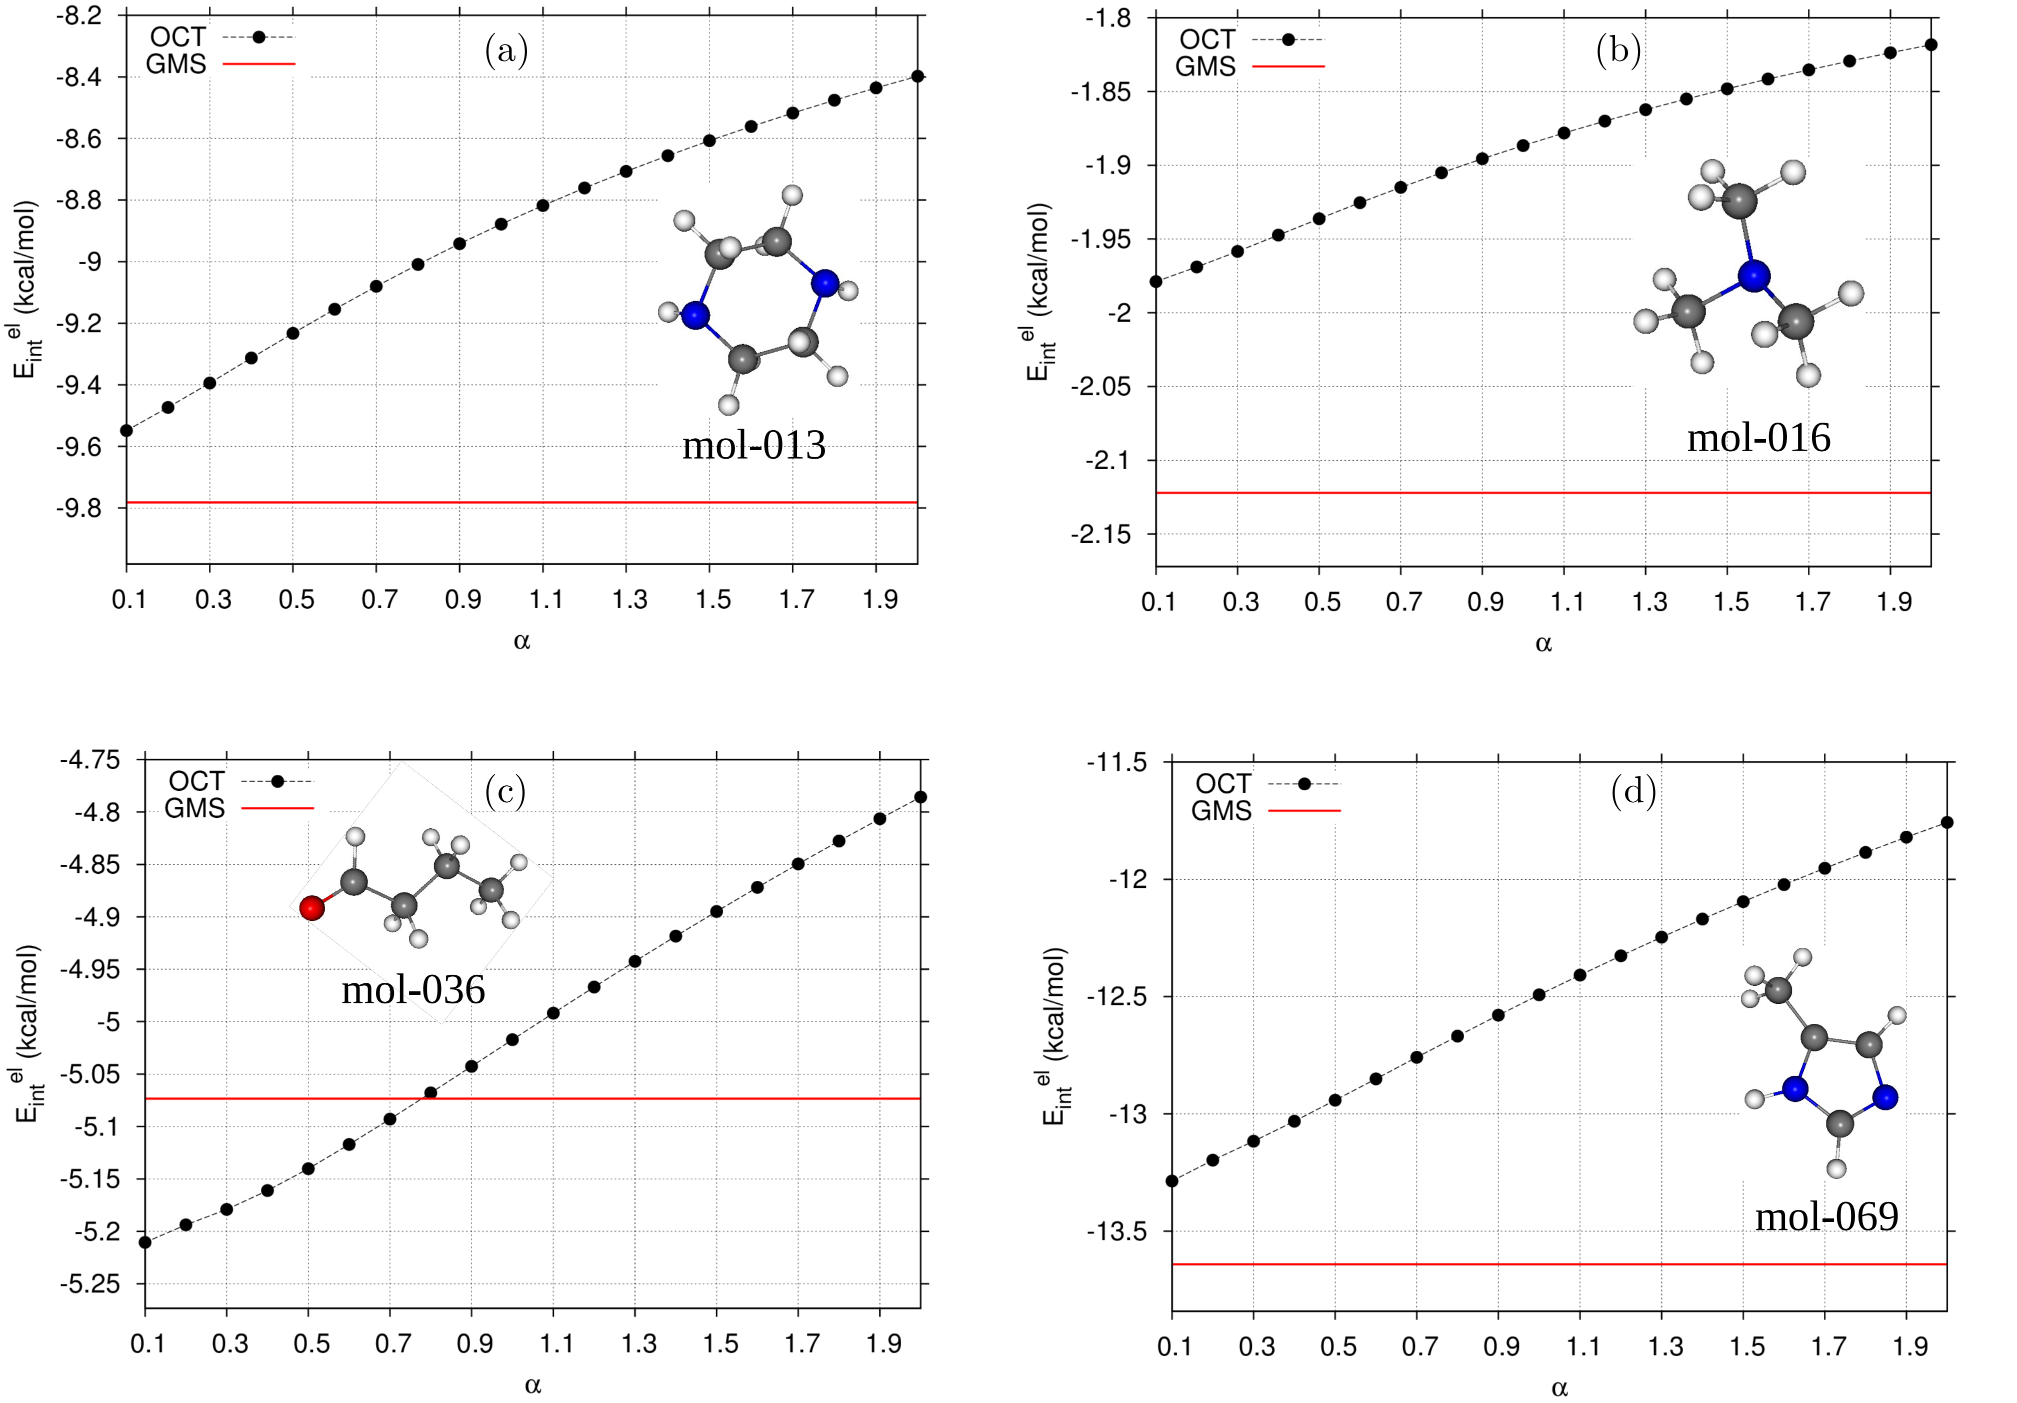


Fig. 1. Calculated electrostatic interaction energy for (a) piperazine, (b) trimethylammine, (c) butanal and (d) 4-methyl-1H-imidazole molecules in water for different values of the parameter α used to regularize solvent reaction potential in real-space.

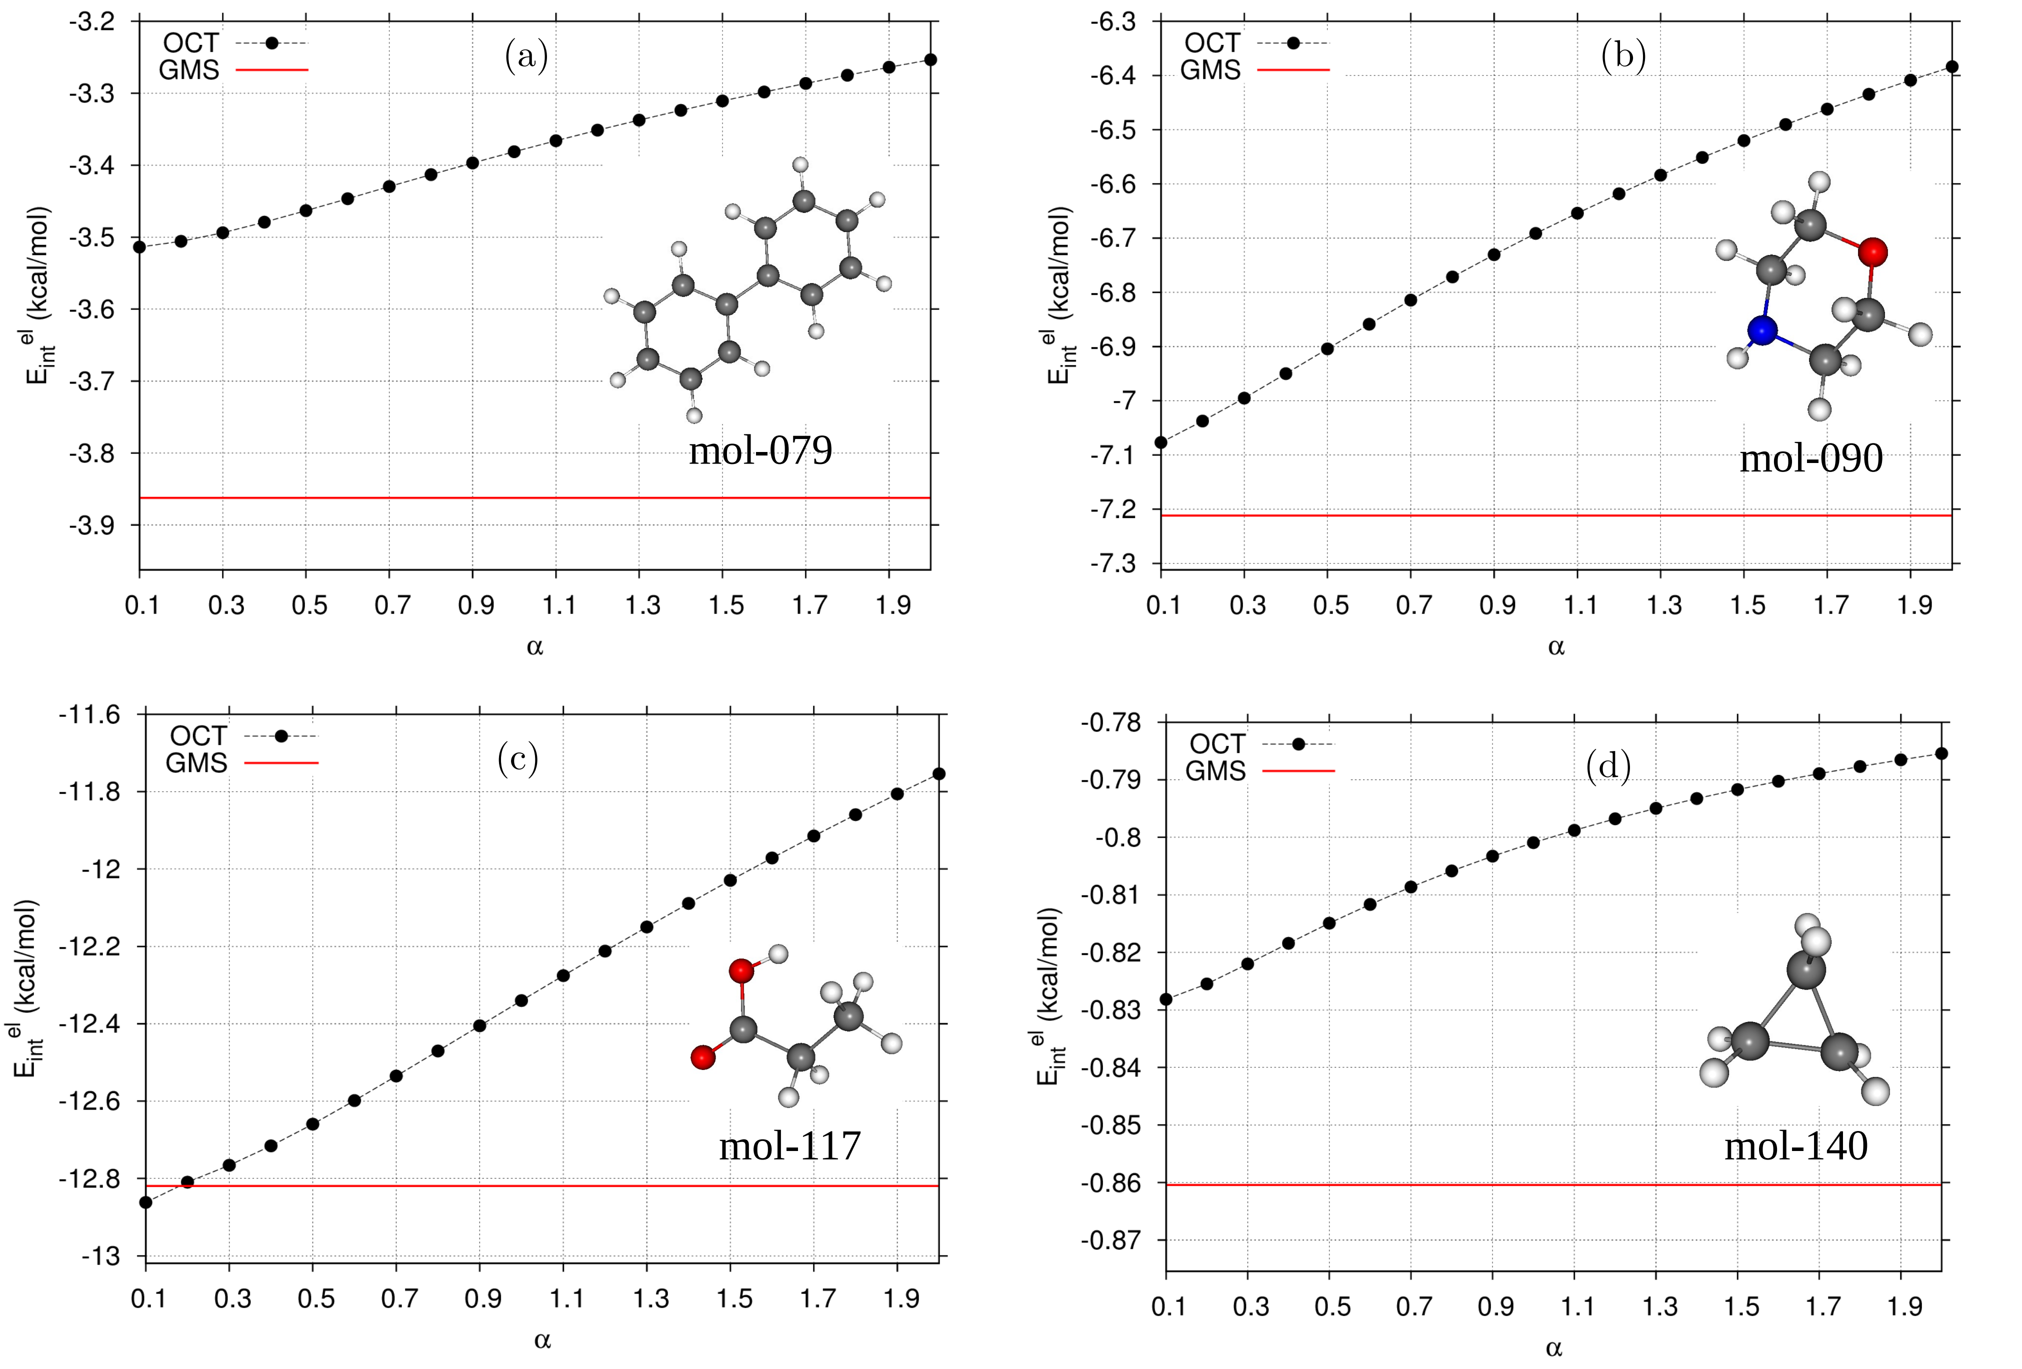


Fig. 2. Calculated electrostatic interaction energy for (a) biphenyl, (b) morpholine, (c) priopionic and (d) cyclopropane molecules in water for different values of the parameter α used to regularize solvent reaction potential in real-space.

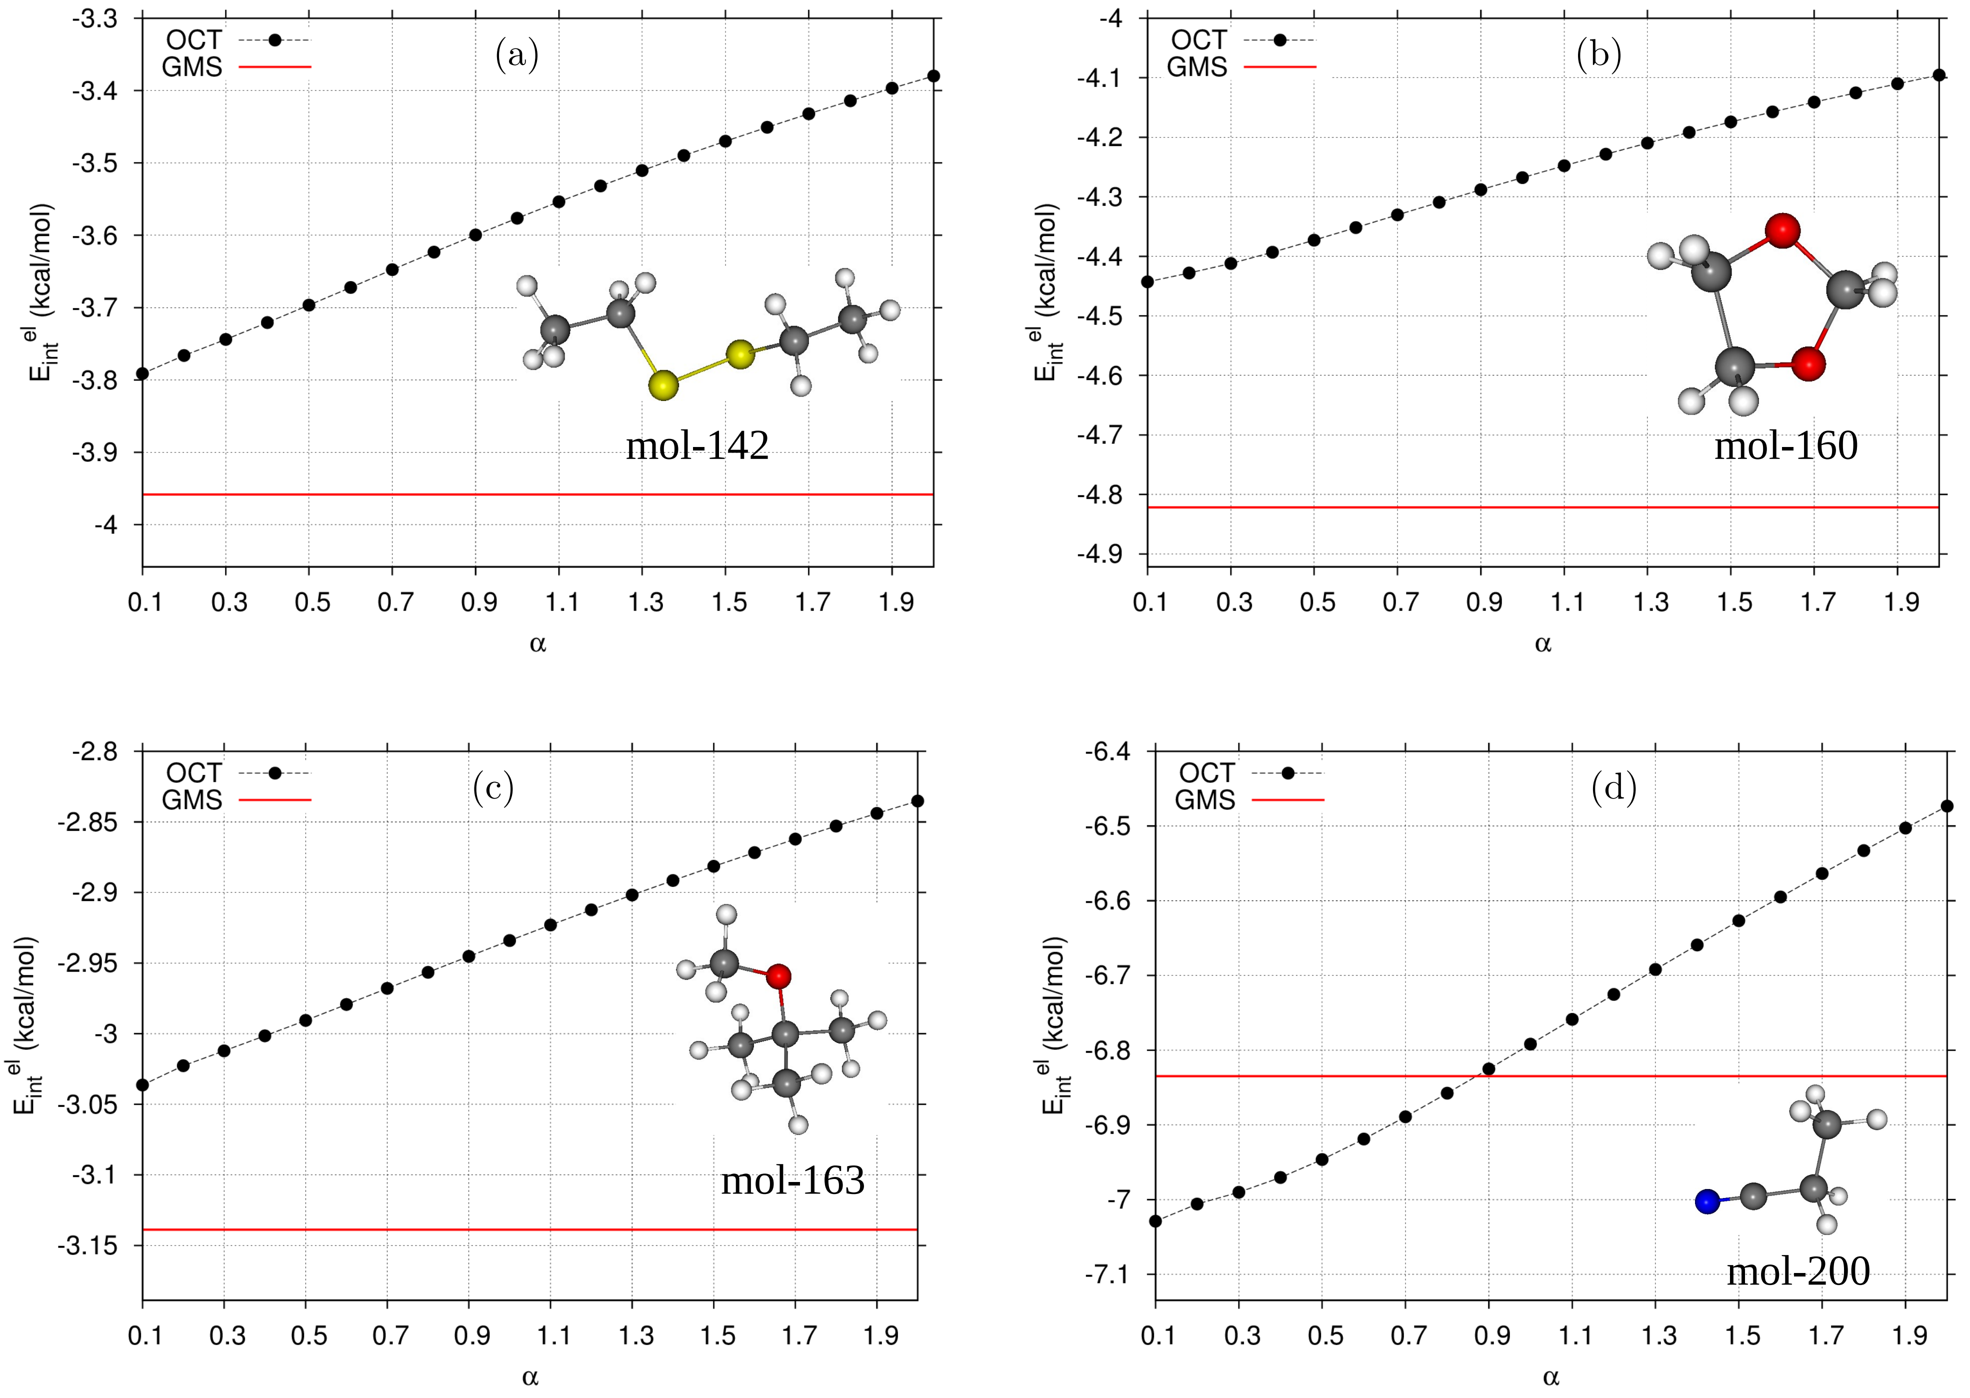


Fig. 3. Calculated electrostatic interaction energy for (a) diethyldisulfide, (b) 1,3-dioxolane, (c) propane-2-methoxy-2-methyl and (d) propiononitrile molecules in water for different values of the parameter α used to regularize solvent reaction potential in real-space.

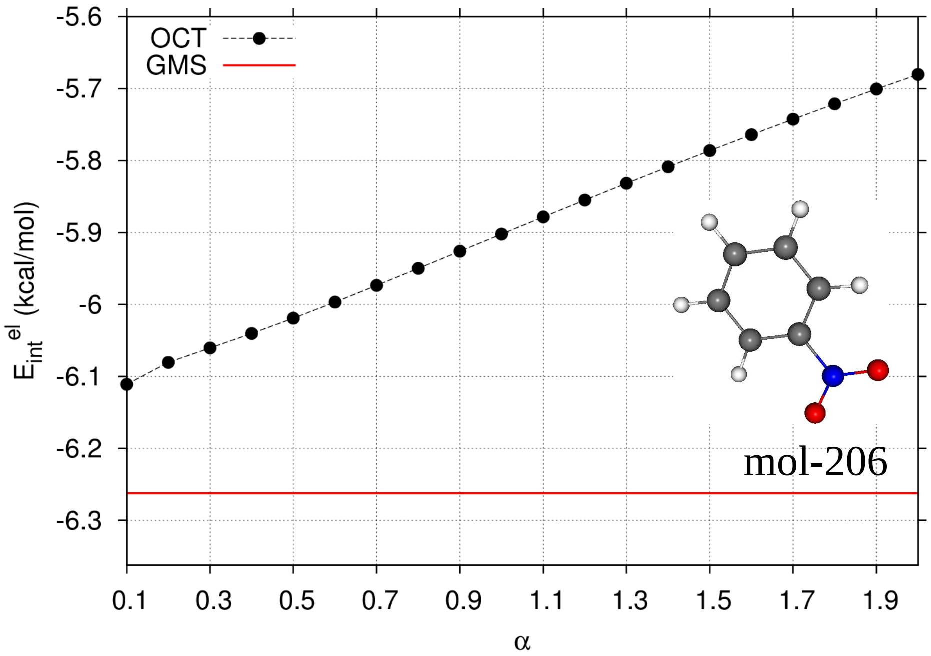


Fig. 4. Calculated electrostatic interaction energy for nitrobenzene molecule in water for different values of the parameter α used to regularize solvent reaction potential in real-space.

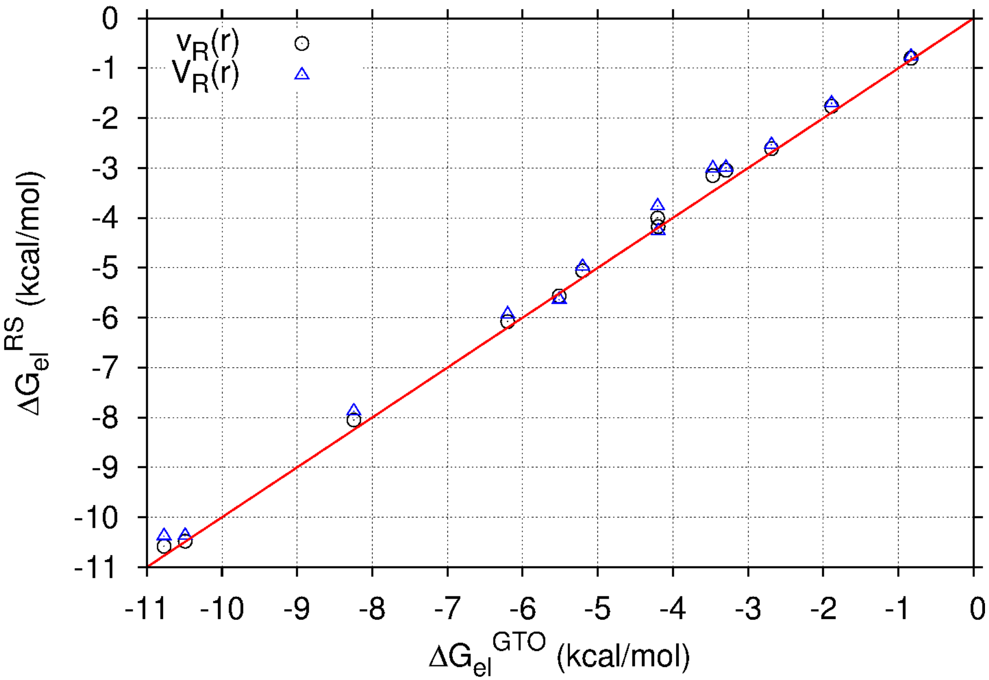


Fig. 5. Electrostatic contribution to the solvation free energy calculated in real-space (RS) with the regularized potential (circles) and without regularization (triangles) for the investigated molecules. Both calculations are correlated with the same results calculated with with GAMESS.

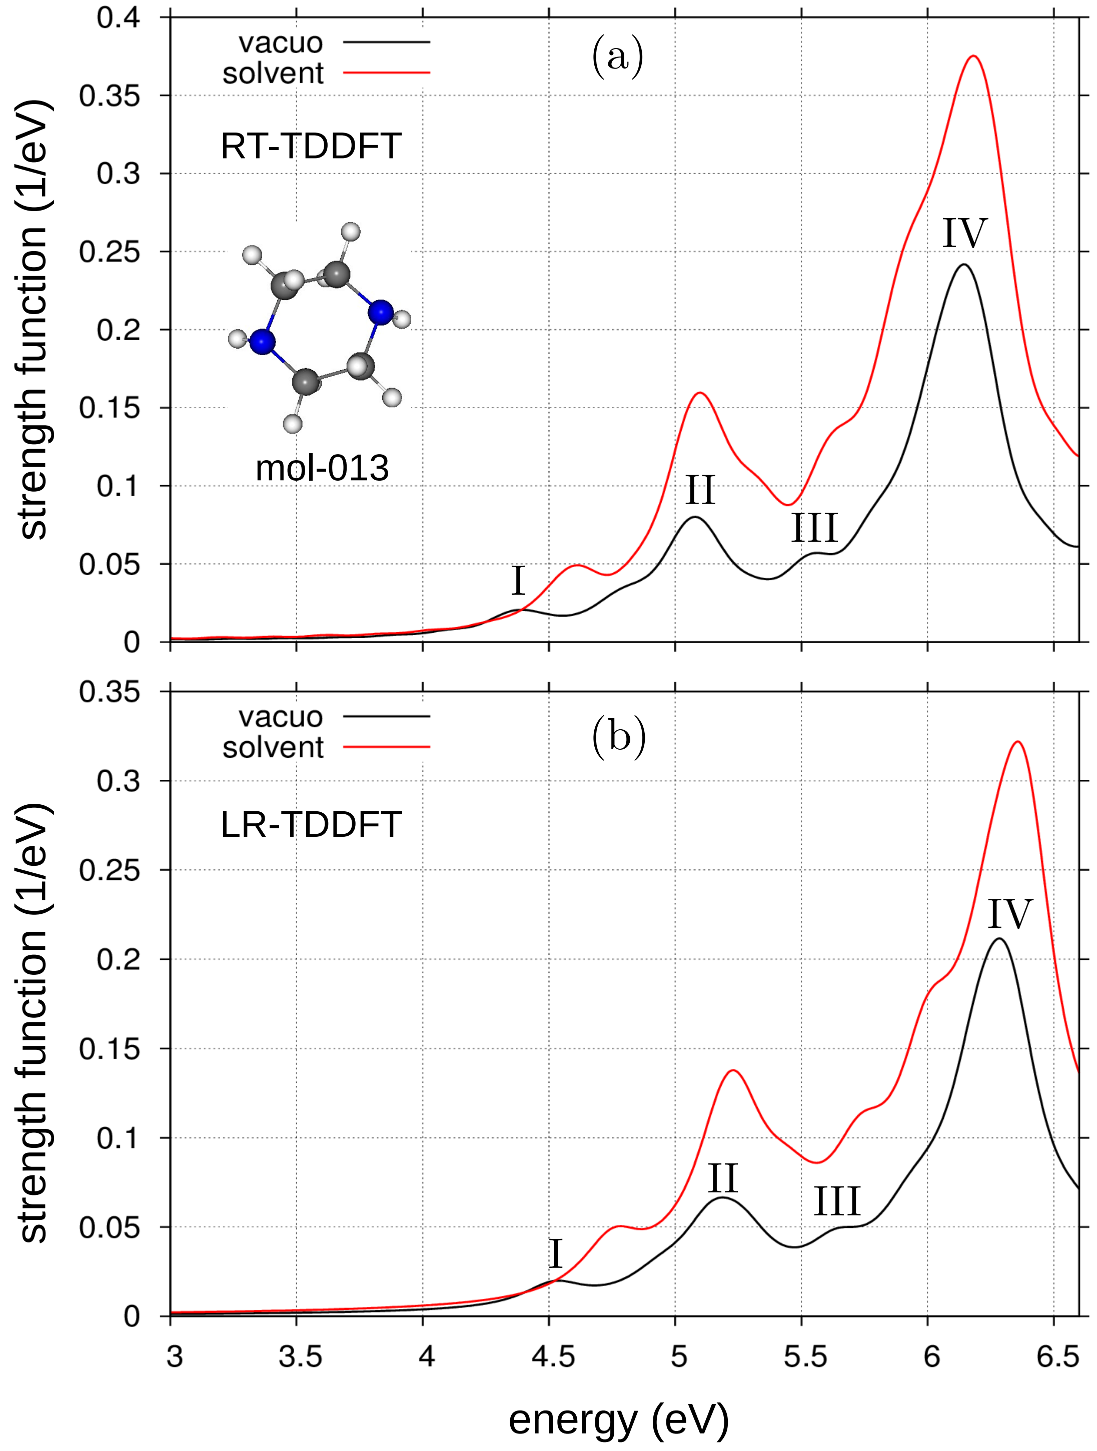


Fig. 6. Absorption spectra of piperazine molecule calculated in vacuo and water. (a) real-time TDDFT (RT-TDDFT) calculations performed with OCTOPUS, (b) linear-response TDDFT (LR-TDDFT) calculations by using GAMESS.

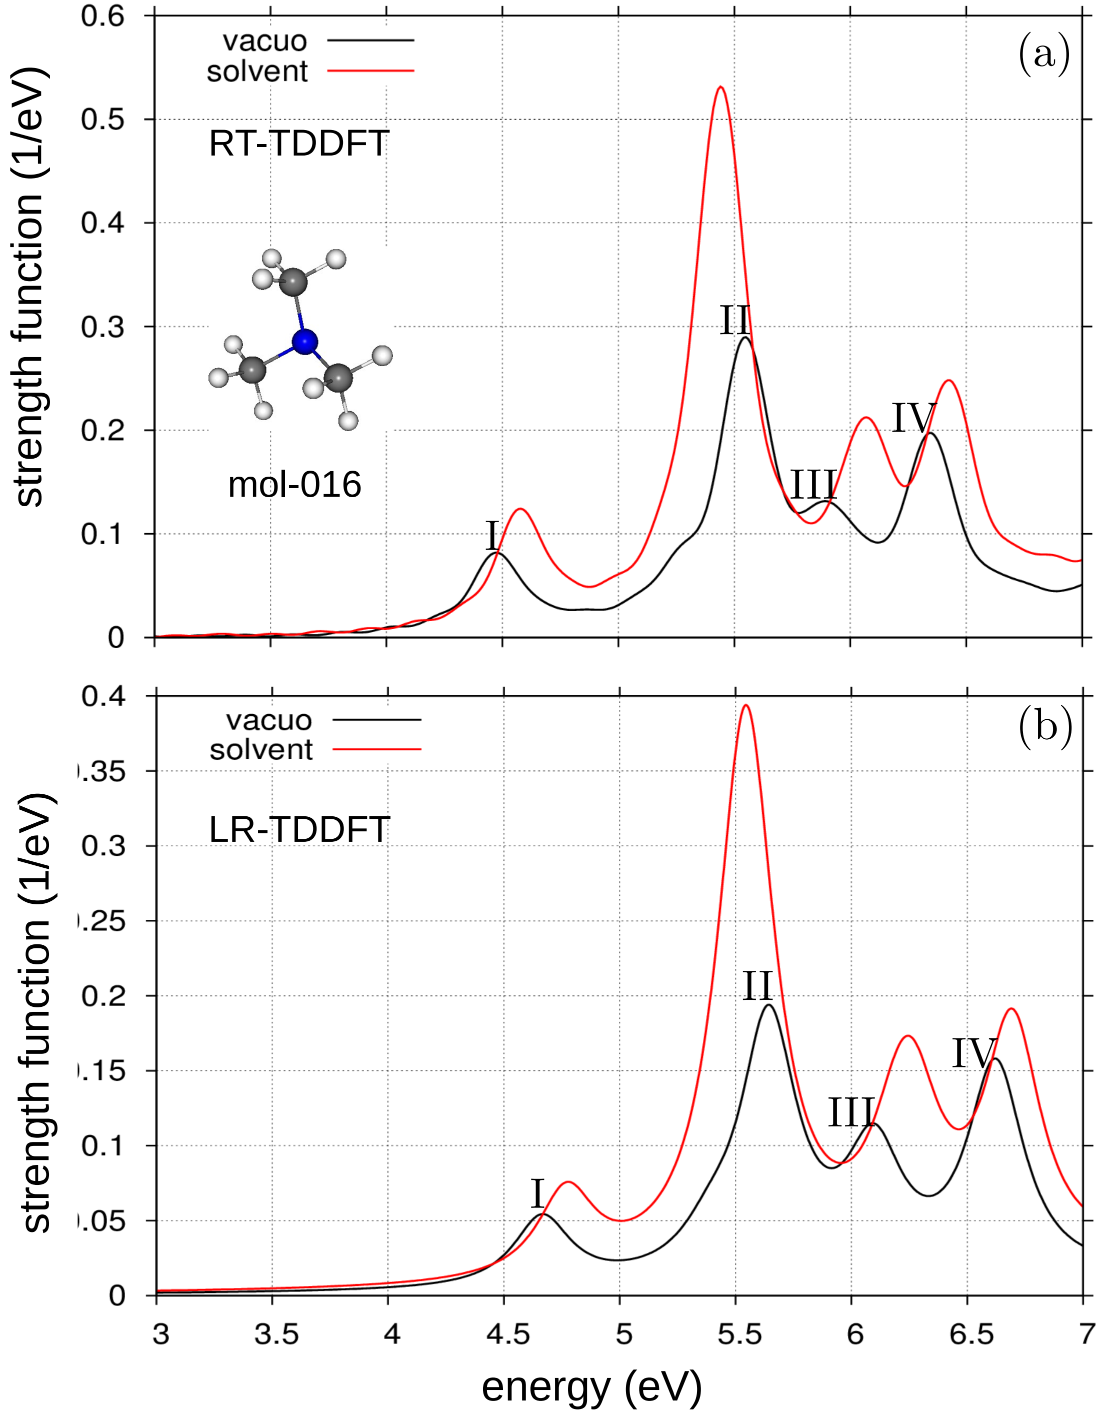


Fig. 7. Absorption spectra of trimethylammine molecule calculated in vacuo and water. (a) real-time TDDFT (RT-TDDFT) calculations performed with OCTOPUS, (b) linear-response TDDFT (LR-TDDFT) calculations by using GAMESS.

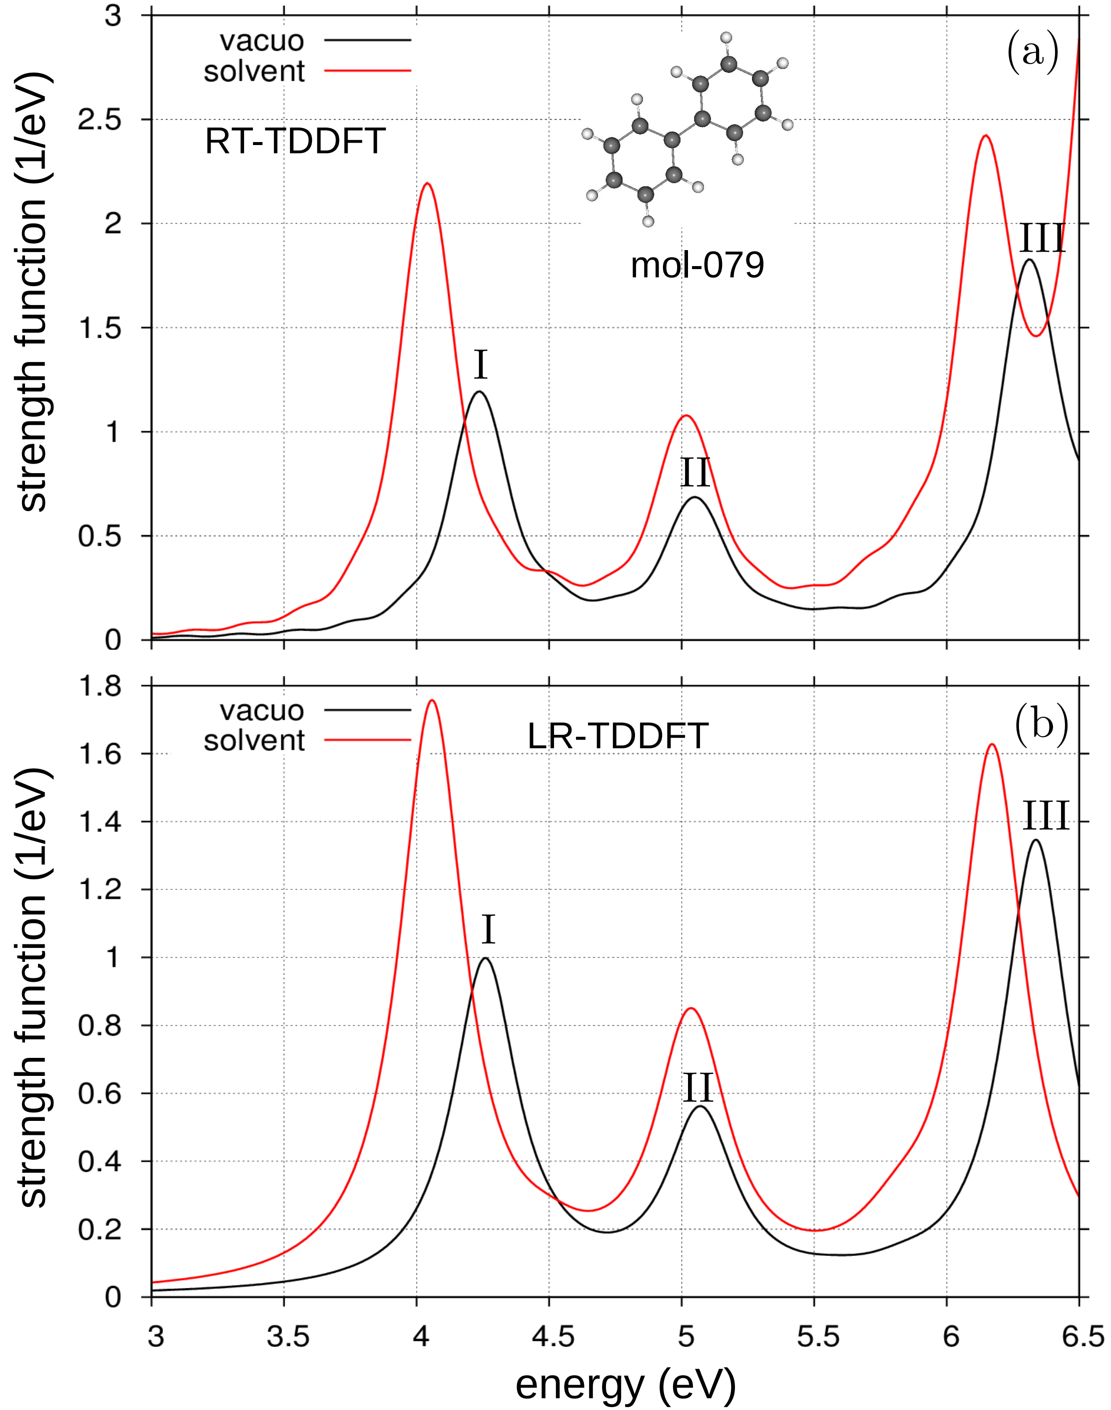


Fig. 8. Absorption spectra of biphenyl molecule calculated in vacuo and water. (a) real-time TDDFT (RT-TDDFT) calculations performed with OCTOPUS, (b) linear-response TDDFT (LR-TDDFT) calculations by using GAMESS.
